# Supplementary material for: The Efficacy of Transfer-based No-box Attacks on Image Watermarking: A Pragmatic Analysis
Source: arXiv:2412.02576 source file (2024-12-03)
Supplement: Supplementary file 1 [file attacks.tex]

\subsection{Examplar No-Box Attacks}

\varun{long story short there are 3 attacks: 1. transfer attacks (and those like it); 2. diffusion purification (and those like it); 3. ones like zhao et al.}

\ql{will remove whichever we are not implementing}

\noindent{\bf Non-learning Distortions:} Single and combined non-learning distortions (like cropping, JPEG noise) are also evaluated in \citet{an2024box} as attack methods. However, \citet{an2024box} shows that the learning-based watermarks they evaluate \texttt{Tree-Ring}. \texttt{Stable Signature}, \texttt{StegaStamp}, \texttt{MBRS}, are generally robust against this type of attacks, though \texttt{MBRS} is not robust to some distortions. 

\varun{same as zhao et al.}
\noindent{\bf Regeneration Attack}
\citet{an2024box} evaluates regeneration attacks \texttt{Regeneration via diffusion}, \texttt{Regeneration via VAE}, \texttt{Regeneration via KL-VAE} where different generation models (Stable Diffusion v1.4, VAE, KL-VAE) are used for denoising without explicitly adding noise to watermarked images. Such attacks are successful on \texttt{Tree Ring}, \texttt{Stable Signature}, and  \texttt{MBRS} but not on \texttt{StegaStamp}. \texttt{Prompt Regeneration} and \texttt{Regeneration via prompted diffusion} in \citet{an2024box} are not considered no-box attacks as they additionally assume prompt information.

\noindent{\bf Diffusion Purification:} Diffusion purification, first proposed in \citet{nie2022diffusion}, and its variants \citep{nie2022diffusion} can also be used to attack image watermarking \citep{saberi2023robustness} \citep{zhao2023invisible}. In this attack, noise is added to the image space or embedding space and then a diffusion or VAE model is used to remove the Gaussian noise, which also removes the watermarking. \texttt{Rinse} \citep{an2024box} takes the same procedure but has multiple cycles of noising and denoising through a pre-trained diffusion model. \texttt{Rinse} can also be combined with regeneration attack by concatenation \citep{an2024box}. However, these methods are limited to low-perturbation watermarks \citep{saberi2023robustness} or invisible watermarks \citep{zhao2023invisible}, and it is unclear if they can evade high-perturbation watermarks like \texttt{StegaStamp} and \texttt{TreeRing}. \footnote{For \texttt{StegaStamp}, \citet{saberi2023robustness} argues it can be evaded by diffusion purification attack, but \citet{zhao2023invisible} argues it is robust; for \texttt{Tree Ring}, \citet{an2024box} argues it can be evaded by regeneration attacks and diffusion purification attacks, while \citet{zhao2023invisible,saberi2023robustness} argues it is robust.}

\varun{same as diffusion purification} \noindent{\bf Controlled Regeneration:} One concurrent work \citep{liu2024image} shares a similar idea, proposing \texttt{CtrlRegen} and \texttt{CtrlRegen+}. \texttt{CtrlRegen} controls the regeneration of watermarked images from clean noise. \texttt{CtrlRegen+} adds noise to latent space and then denoise before controlled generation. Semantic control and spatial control help improve quality and enable it to also evade semantic/high perturbation watermarks like \citep{wen2023tree}, yet the cost is to train two control networks using 10 million and 118k image-canny pairs, which is computationally expensive. Diffusion purification-based methods, \texttt{CtrlRegen}, and \texttt{CtrlRegen+} also have no direct control to ensure the attacked image is within specific budgets from the input watermarked images. 

\varun{appendix}
\noindent{\bf Embedding Attacks:} Embedding attacks in \citet{an2024box} crafts adversarial image $x_{adv}$ to diverge its embedding from the original image $x_{wm}$ but within $l_{inf}$ perturbation budget in the image space. This is successful on \texttt{Tree-Ring} but not on \texttt{Stable Signature}, \texttt{StegaStamp}, and \texttt{MBRS}.

\varun{appendix}
\noindent{\bf StegaAnalysis:} In contrast, \citet{yang2024steganalysis} tries to extract watermark patterns from watermarked and unwatermarked images  \varun{assumes access to unwatermarked images} to subtract the extracted version for removal, but its success is mainly limited to content-agnostic watermarks, which are more high-perturbation and perceptible.

\varun{appendix}
\noindent{\bf Surrogate Detector Attacks:} \texttt{AdvCls-Real\&WM} from \citet{an2024box} is the only attack considered no-box within their surrogate detector attacks as it uses watermarked images and unwatermarked images \varun{assumes access to unwatermarked images} to train a surrogate detector and unwatermarked images are sampled ImageNet dataset rather than the victim model. Then attacks are conducted on the surrogate model. However, \citet{an2024box} finds it is only successful on \texttt{Tree-Ring} but not \texttt{Stable Signature}, \texttt{StegaStamp}, and \texttt{MBRS}.

\noindent{\bf UnMarker:} Another concurrent work \citep{kassis2024unmarker} uses spectral optimization and has successful evasion, but cropping is one necessary component, and quality degradation is visible, which can be undesirable in some scenarios and fails norm constraints, and the computation cost is also not cheap.  \varun{seems black box based on s5 in \url{https://arxiv.org/pdf/2405.08363}}

\noindent{\bf Transfer:} Transfer attack is another feasible way \citep{hu2024transfer} and what we focus on. It takes the intuition that if surrogate models' decoded messages are flipped by adding perturbation, the target model's decoded message can also be disturbed. They use optimization techniques to find such an adversarial perturbation. Despite generally successful evasion in the reported evaluation, we will see that it requires a lot of surrogate models with limited architecture differences between the surrogate models. 

\vspace{1mm}
\noindent{\bf {Smoothing}:}~\citet{jiang2024certifiably} propose a certified image watermarking technique (i.e., with guarantees against removal and spoofing attacks). It is implemented by adding noise to augment the image before sending it to the decoder, then the final detection result comes from aggregating the detection results on augmented images.  The best choice of aggregation they find is to take the median of the Bit-wise Accuracy for augmented images. 

A more formal representation is as follows:

\begin{enumerate}
    \item First, compute the individual Bit-wise Accuracy (\texttt{BA}) for each noisy image:
    \[
    \texttt{BA}_i = \texttt{BA}(s, \texttt{Dec}(x_{wm} + \varepsilon_i)), \quad i = \{1, 2, \dots, N \}
    \]
    where \( N \) is the number of noisy images, and \( \epsilon_i \sim \mathcal{N}(0, \sigma^2 I) \) are i.i.d. Gaussian noise variables with \( \sigma \) as the noise strength hyperparameter.

    \item Next, compute the median of these accuracy values:
    \[
    \texttt{BA}_m = \texttt{median}(\texttt{BA}_1, \texttt{BA}_2, \dots, \texttt{BA}_N)
    \]

    \item Finally, the detection outcome is based on \( \texttt{BA}_m \):
    \[
    \texttt{Det}(s, \texttt{Dec}(x_{wm})) =
    \begin{cases} 
        1, & \text{if } \texttt{BA}_m \geq 1 - \delta \text{ or } \texttt{BA}_m \leq \delta \\
        0, & \text{otherwise}
    \end{cases}
    \]
\end{enumerate}

Such a method only changes detection and is model-agnostic, which can be used to achieve certified robustness for existing watermarking methods like \texttt{StegaStamp} and \texttt{HiDDeN} in plug-and-play style.  While it enables certified robustness, it does not change the model itself, and it hardly shows improved robustness facing optimization-based transfer attack~\cite{hu2024transfer}. Consequently, we do not include this method in our experiment.

%Considering the practice and limited exploration, we focus on the no-box setting.
